# Supplementary material for: Is the brain macroscopically linear? A system identification of resting state dynamics
Source: arXiv:2012.12351 ancillary file (2021-08-11)
Supplement: Supplementary file 1 [file Supplementary_Material.pdf]

**Supplementary Material for**  
**“Is the brain macroscopically linear?”**  
**A system identification of resting state dynamics”**

Erfan Nozari<sup>1</sup>, Jennifer Stiso<sup>2,3</sup>, Lorenzo Caciagli<sup>2</sup>, Eli J. Cornblath<sup>2,3</sup>, Xiaosong He<sup>2</sup>,  
Maxwell A. Bertolero<sup>2</sup>, Arun S. Mahadevan<sup>2</sup>, George J. Pappas<sup>4</sup>, and  
Danielle S. Bassett<sup>2,4,5,6,7,8,\*</sup>

<sup>1</sup>*Department of Mechanical Engineering, University of California, Riverside, CA, USA*

<sup>2</sup>*Department of Bioengineering, University of Pennsylvania, Philadelphia, PA, USA*

<sup>3</sup>*Department of Neuroscience, University of Pennsylvania, Philadelphia, PA, USA*

<sup>4</sup>*Department of Electrical and Systems Engineering, University of Pennsylvania, Philadelphia, PA, USA*

<sup>5</sup>*Department of Physics & Astronomy, University of Pennsylvania, Philadelphia, PA, USA*

<sup>6</sup>*Department of Neurology, University of Pennsylvania, Philadelphia, PA, USA*

<sup>7</sup>*Department of Psychiatry, University of Pennsylvania, Philadelphia, PA, USA*

<sup>8</sup>*Santa Fe Institute, Santa Fe, NM, USA*

<sup>\*</sup>*Corresponding author (email: dsb@seas.upenn.edu)*

## Supplementary Note 1: Effect of Bandpass Filtering on System Identification and the Detection of Nonlinearity

A standard step in the preprocessing of resting state fMRI time series is bandpass filtering, typically over the range  $[0.01, 0.08]$  Hz [1], to reduce the contribution of non-neuronal sources on the signal and improve the SNR. In this work, however, we purposefully avoided this step. In the following, we discuss in detail the role and effects of pre-filtering in this rather unconventional context of system identification and, in particular, detection of nonlinear dynamics.

1. First, bandpass filtering (or any linear filtering for this matter) has no effect on the fitting or evaluation of linear models. The reason, in short, is the commuting property of linear systems. More specifically, any linear system including all of the ones used in this work can be written in the impulse-response form [2]

$$\mathbf{y}(t) = \mathbf{G}(q)\mathbf{e}(t),$$

where  $\mathbf{G}$  is the transfer matrix

$$\mathbf{G}(q) = \begin{bmatrix} G_{11}(q) & G_{12}(q) & \cdots \\ G_{21}(q) & G_{22}(q) & \cdots \\ \vdots & \vdots & \ddots \end{bmatrix}$$

such that for any  $i$  and  $j$

$$G_{ij}(q) = g_{ij}(0) + g_{ij}(1)q^{-1} + g_{ij}(2)q^{-2} + \cdots$$

Here,  $g_{ij}(t)$  is the impulse response from the the  $j$ th input  $e_j(t)$  to the  $i$ th output  $y_i(t)$ , and  $q$  is the standard shift operator such that  $q^{-1}s(t) = s(t-1)$  for any signal  $s(t)$  [3]. Recall that  $\mathbf{y}(t)$  is the BOLD time series without bandpass filtering, as used in the main text, and let

$$F(q) = f(0) + f(1)q^{-1} + f(2)q^{-2} + \cdots$$

be any linear filter, including the bandpass filter used in common preprocessing pipelines. Assume, without loss of generality, that  $f(0) \neq 0$  (an almost identical argument can be given if  $f(0)$  or any number of the first terms in  $F(q)$  are zero, simply by factoring out enough powers of  $q^{-1}$ ). The output of the filter is

$$\mathbf{z}(t) = F(q)\mathbf{y}(t) = F(q)\mathbf{G}(q)\mathbf{e}(t).$$

It then immediately follows from the prediction error framework [3] that the one step ahead prediction error of  $\mathbf{z}(t)$  is given by

$$\begin{aligned} \mathbf{z}(t) - \hat{\mathbf{z}}(t|t-1) &= f(0)\mathbf{G}^{-1}(q)F^{-1}(q)\mathbf{z}(t) \\ &= f(0)\mathbf{G}^{-1}(q)\mathbf{y}(t) \\ &= f(0)[\mathbf{y}(t) - \hat{\mathbf{y}}(t|t-1)]. \end{aligned}$$

In other words, the prediction error of  $\mathbf{z}(t)$  is identical to the prediction error of  $\mathbf{y}(t)$ , except for a constant factor equal to the instantaneous gain of the filter. Therefore, not only is fitting a model by minimizing the prediction error of  $\mathbf{z}(t)$  identical to fitting a model by minimizing the prediction error of  $\mathbf{y}(t)$ , but the cross-validated  $R^2$  (up to a fixed constant) and residual whiteness of these models are also identical.

This argument clearly fails for nonlinear systems. Indeed, fitting a nonlinear model on  $\mathbf{z}(t)$  can result in a different model with different  $R^2$  and residual whiteness than the same model fit on  $\mathbf{y}(t)$ . The critical point, however, is that the linear filter  $F(q)$  cannot generate nonlinearity, while it can certainly weaken and even eliminate it. We explain these two points in more detail next.

2. Assume, first, that the dynamics of  $\mathbf{y}(t)$  are truly linear, as seems to be the case from our analysis in the main text. Then, the relationship between  $\Delta\mathbf{y}(t)$  and  $\mathbf{y}(t-1)$  (as random vectors) is linear. By definition, if the relationship between two random vectors  $\mathbf{u}$  and  $\mathbf{v}$  is linear, they can be written in the form

$$\begin{bmatrix} \mathbf{u} \\ \mathbf{v} \end{bmatrix} = \begin{bmatrix} \mathbf{A}_{11} & \mathbf{A}_{12} \\ \mathbf{A}_{21} & \mathbf{A}_{22} \end{bmatrix} \begin{bmatrix} \mathbf{e}_1 \\ \mathbf{e}_2 \end{bmatrix} \quad (\text{S1})$$

where  $\mathbf{A}$  is an appropriate matrix and  $\mathbf{e}_1$  and  $\mathbf{e}_2$  are independent. Now let  $\mathbf{u}_F$  be the result of applying a linear filter  $F(q)$  to (the samples of)  $\mathbf{u}$ . In other words, if  $N$  is the order of an (arbitrarily accurate) FIR approximation of  $F(q)$ ,

$$\mathbf{u}_F = [\mathbf{u}_1 \quad \mathbf{u}_2 \quad \cdots \quad \mathbf{u}_N] \begin{bmatrix} f(0) \\ f(1) \\ \vdots \\ f(N-1) \end{bmatrix} = [\mathbf{u}_1 \quad \mathbf{u}_2 \quad \cdots \quad \mathbf{u}_N] \mathbf{f} \quad (\text{S2})$$

where  $f(t)$  is the impulse response of  $F(q)$  and  $\mathbf{u}_1, \mathbf{u}_2, \dots, \mathbf{u}_N$  are identically distributed (but not necessarily independent) samples of  $\mathbf{u}$ . From Eq. (S1),

$$[\mathbf{u}_1 \quad \mathbf{u}_2 \quad \cdots \quad \mathbf{u}_N] = [\mathbf{A}_{11} \quad \mathbf{A}_{12}] \begin{bmatrix} \mathbf{e}_{1,1} & \mathbf{e}_{1,2} & \cdots & \mathbf{e}_{1,N} \\ \mathbf{e}_{2,1} & \mathbf{e}_{2,2} & \cdots & \mathbf{e}_{2,N} \end{bmatrix} \quad (\text{S3})$$

where  $\mathbf{e}_{1,1}, \dots, \mathbf{e}_{1,N}$  are identically distributed (but not necessarily independent) samples of  $\mathbf{e}_1$ , similarly for  $\mathbf{e}_2$ . Note that each  $\mathbf{e}_{1,t}$  is still independent from each  $\mathbf{e}_{2,s}$  by definition. Substituting Eq. (S3) into Eq. (S2) thus gives

$$\begin{aligned} \mathbf{u}_F &= [\mathbf{A}_{11} \quad \mathbf{A}_{12}] \begin{bmatrix} \mathbf{e}_{1,1} & \mathbf{e}_{1,2} & \cdots & \mathbf{e}_{1,N} \\ \mathbf{e}_{2,1} & \mathbf{e}_{2,2} & \cdots & \mathbf{e}_{2,N} \end{bmatrix} \mathbf{f} \\ &= [\mathbf{A}_{11} \quad \mathbf{A}_{12}] \begin{bmatrix} \mathbf{e}_{1,F} \\ \mathbf{e}_{2,F} \end{bmatrix} \end{aligned}$$

where  $\mathbf{e}_{1,F}$  and  $\mathbf{e}_{2,F}$  are filtered versions of  $\mathbf{e}_1$  and  $\mathbf{e}_2$  and, still, independent of each other. Following the same steps for  $\mathbf{v}$ , we get

$$\begin{bmatrix} \mathbf{u}_F \\ \mathbf{v}_F \end{bmatrix} = \begin{bmatrix} \mathbf{A}_{11} & \mathbf{A}_{12} \\ \mathbf{A}_{21} & \mathbf{A}_{22} \end{bmatrix} \begin{bmatrix} \mathbf{e}_{1,F} \\ \mathbf{e}_{2,F} \end{bmatrix}$$

showing that  $\mathbf{u}_F$  and  $\mathbf{v}_F$  are still linearly related after filtering. This is indeed expected since a linear filter cannot generate nonlinear dependence between two signals that are originally linearly related.

3. Now assume, in contrast, that the dynamics of  $\mathbf{y}(t)$  is in fact nonlinear and we filter  $\mathbf{y}(t)$  to get  $\mathbf{z}(t) = F(q)\mathbf{y}(t)$ . The best that can happen, as far as detecting nonlinearity is concerned, is that the dynamics of  $\mathbf{z}(t)$  remain nonlinear. However, it is possible that  $F(q)$  weakens or completely averages out the nonlinearities in  $\mathbf{y}(t)$ , as we saw in the main text. In fact, the common bandpass filter over  $[0.01, 0.08]$  Hz (compared to a Nyquist frequency of  $1/2\text{TR} \simeq 0.7$  Hz) is strongly lowpass and involves significant averaging over time.

In conclusion, while bandpass filtering has no effect on linear models and preserves linearity of time series, it can well weaken/eliminate any nonlinearity in the time series. Therefore, regardless of how much “cleaner” bandpass-filtered data might be, finding no nonlinearity before bandpass filtering, as pursued in the main text, is a stronger statement than the same finding would be if obtained after bandpass filtering.

## Supplementary References

- [1] R. Ciric, A. F. Rosen, G. Erus, M. Cieslak, A. Adebimpe, P. A. Cook, D. S. Bassett, C. Davatzikos, D. H. Wolf, and T. D. Satterthwaite, “Mitigating head motion artifact in functional connectivity mri,” *Nature protocols*, vol. 13, no. 12, pp. 2801–2826, 2018.
- [2] A. V. Oppenheim, A. S. Willsky, and S. H. Nawab, *Signals and Systems*, ser. Prentice-Hall signal processing series. Prentice Hall, 1997. [Online]. Available: <https://books.google.com/books?id=LwQqAQAAMAAJ>
- [3] L. Ljung, “System identification: theory for the user,” *PTR Prentice Hall, Upper Saddle River, NJ*, pp. 1–14, 1999.

## Supplementary Figures

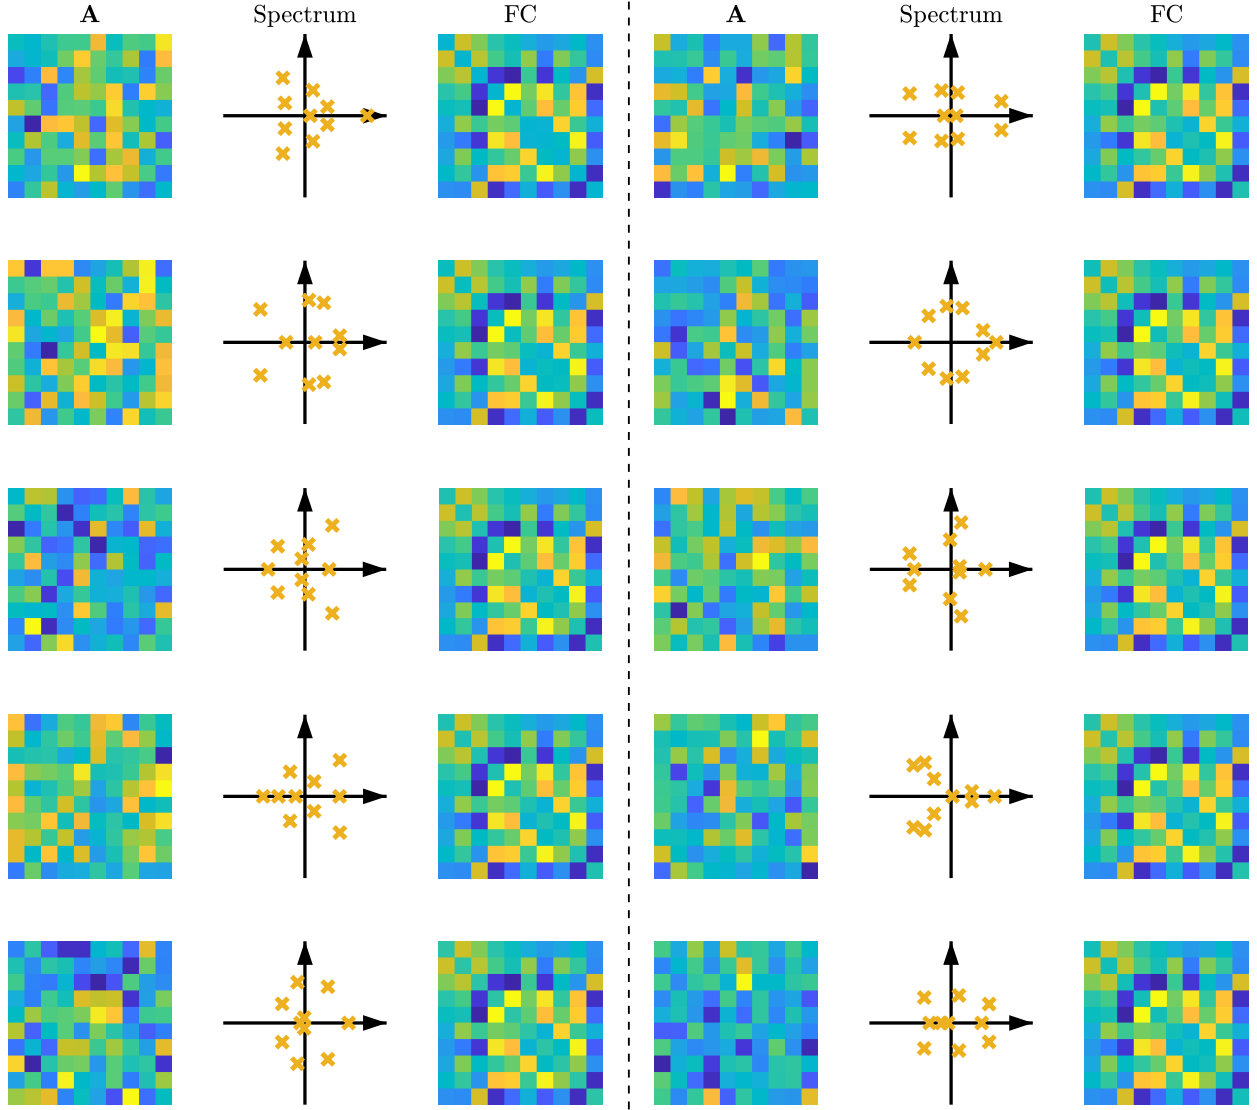

**Supplementary Figure 1: Different systems can produce almost identical functional connectivity (FC).**

Ten different systems of the form  $\mathbf{y}(t) = \mathbf{A}\mathbf{y}(t-1) + \mathbf{e}(t)$  are shown with completely different  $\mathbf{A}$  matrices and spectra (eigenvalues of  $\mathbf{A}$ ), but almost identical FC matrices. The Pearson correlation coefficient between all pairs of FCs is 1.0000 while the absolute value of the Pearson correlation coefficients between the  $\mathbf{A}$  matrices range from a minimum of 0.0023 to a maximum of 0.36. All systems were driven by independent and randomly generated noise sequences  $\mathbf{e}(t)$ . In the figures, the diagonal entries of the FC matrices (which are by definition equal to 1) are set 0 to increase color resolution.

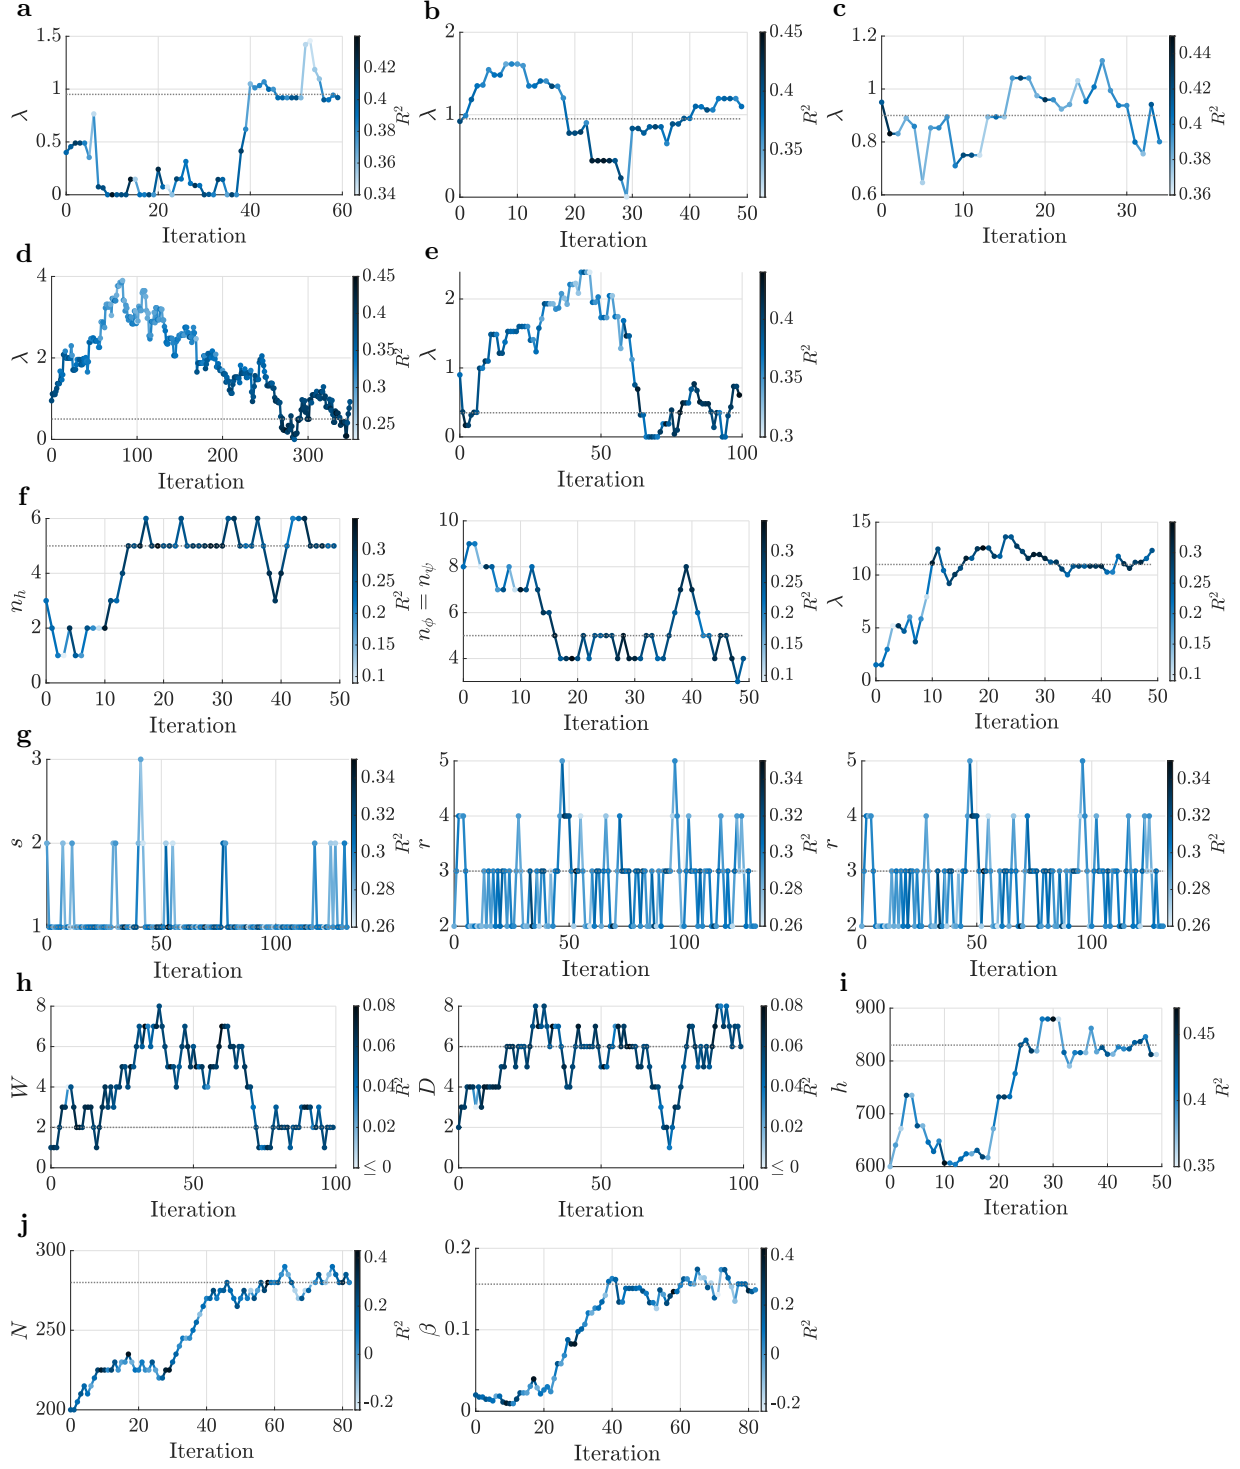

**Supplementary Figure 2: Hyper-parameter tuning of linear and nonlinear model families for fMRI.**

For each parametric family of models, its hyper-parameters were simultaneously optimized using stochastic gradient descent (SGD, see Methods) to select the model with the highest cross-validated  $R^2$  within that model family. (a) Linear (sparse); (b) AR-2 (sparse); (c) VAR-2 (sparse); (d) AR-3 (sparse); (e) VAR-3 (sparse); (f) Linear w/ HRF; (g) Subspace; (h) DNN; (i) Manifold; (j) MMSE (scalar). Each panel shows the evolution of the hyper-parameter(s) of one model family during the SGD iterations, color-coded with the value of  $R^2$  at each iteration, and the hyper-parameter value(s) selected as optimal (dotted gray lines, also given in Table 1 in the main text). Note that the hyper-parameter(s) are not expected to converge to a fixed (optimal) value, but rather to fluctuate around it due to the stochastic nature of SGD and the natural variability of data segments.

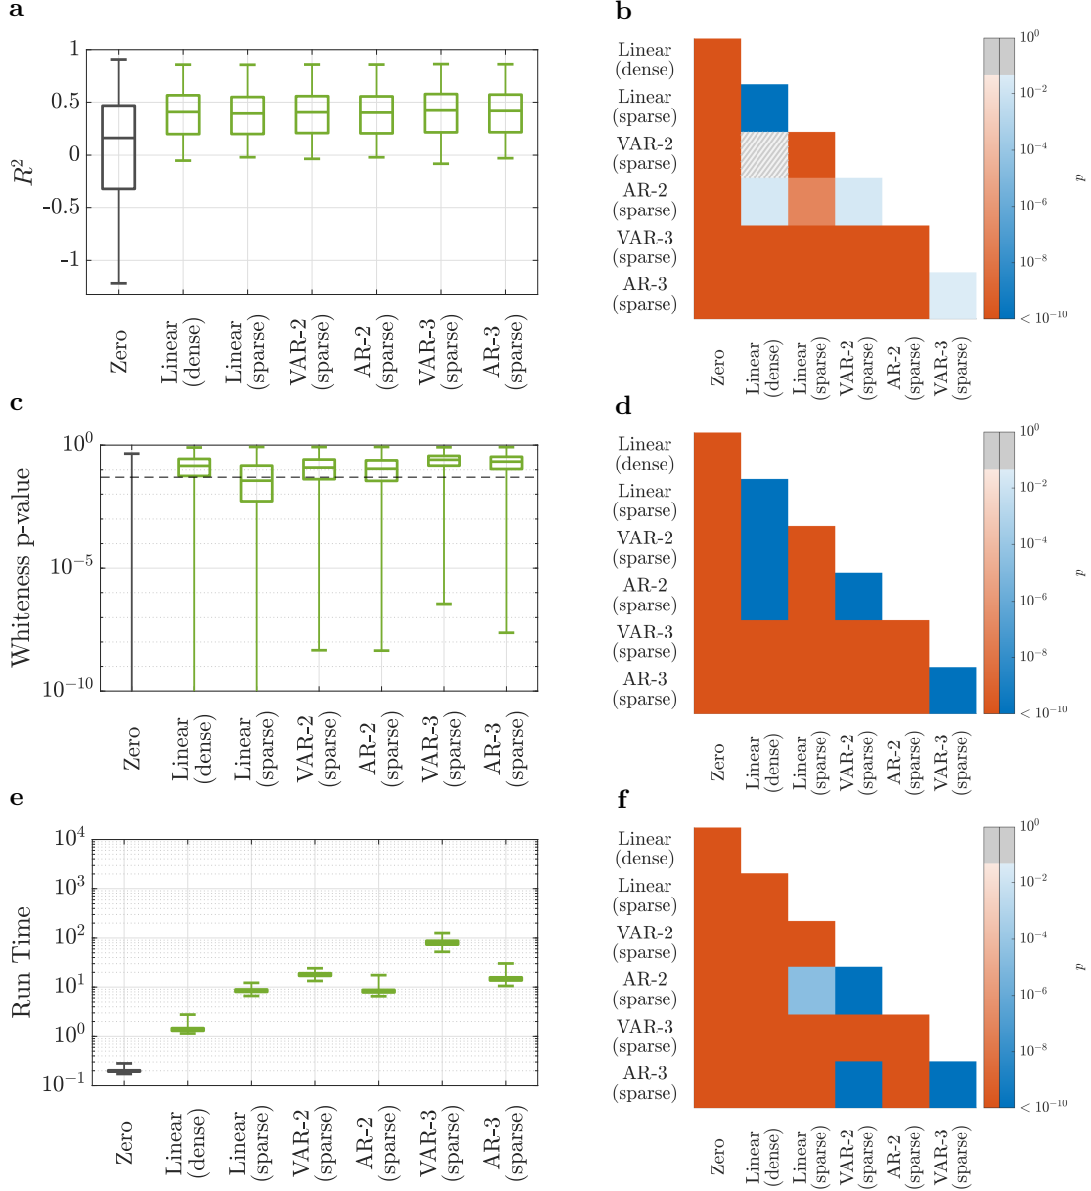

**Supplementary Figure 3: The effects of the number of lags and sparsity patterns on the prediction accuracy and computational complexity of linear AR models of rsfMRI.** Panels parallel those in Figure 2 in the main text and the descriptions of method acronyms are given in Table 1 therein. Generally, the number of lags and sparsity patterns have little effect on the prediction accuracy of linear AR models for rsfMRI data (in contrast to rsiEEG data, as explained in the main text), as seen from panel (a). The estimates of statistical significance in panel (b) are to a great extent due to the large sample size ( $700 \times 116$ ). However, increasing the number of regressors, both by increasing the number of AR lags and by allowing for off-diagonal entries of all lags (‘VAR’ models), does lead to a non-trivial improvement in the whiteness of residuals, even though is often accompanied by non-trivial increases in model complexity and computation time as well.

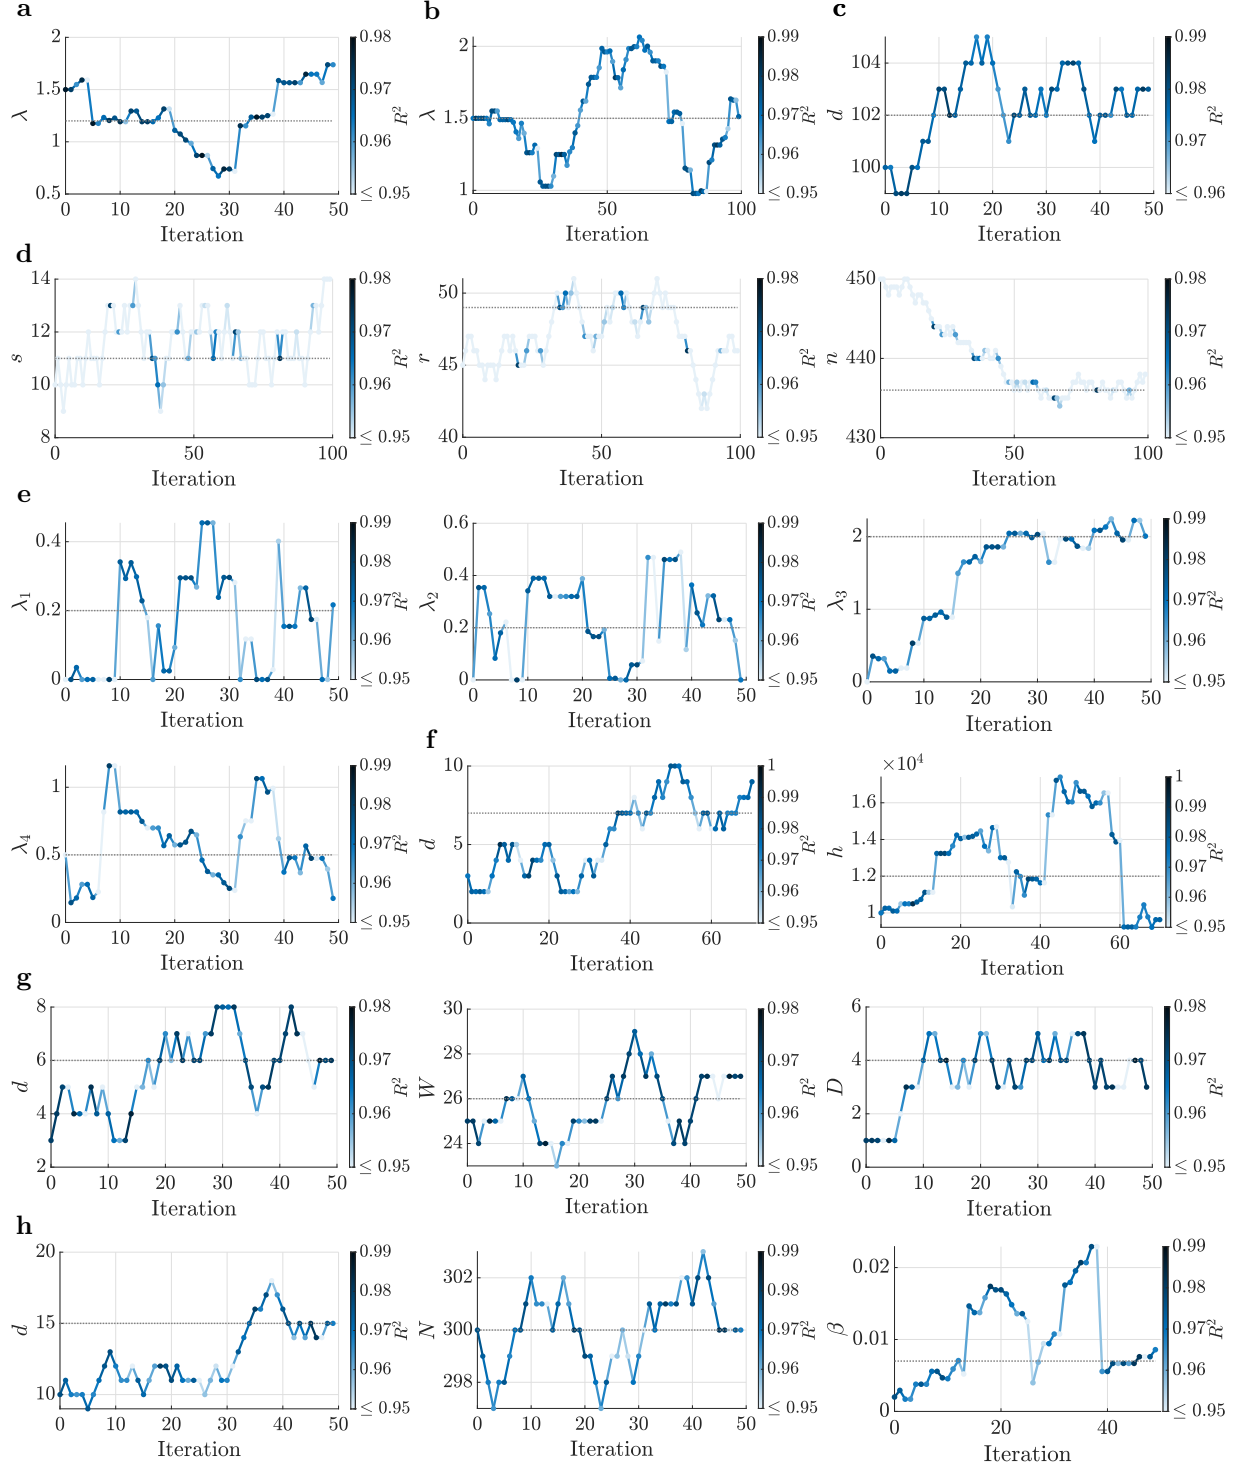

**Supplementary Figure 4: Hyper-parameter tuning of linear and nonlinear model families for iEEG.** (a) Linear (sparse); (b) AR-100 (sparse); (c) AR-100 (scalar); (d) Subspace; (e) NMM; (f) Manifold; (g) DNN; (h) MMSE (scalar). Details and interpretations are the same as Supplementary Figure 2.

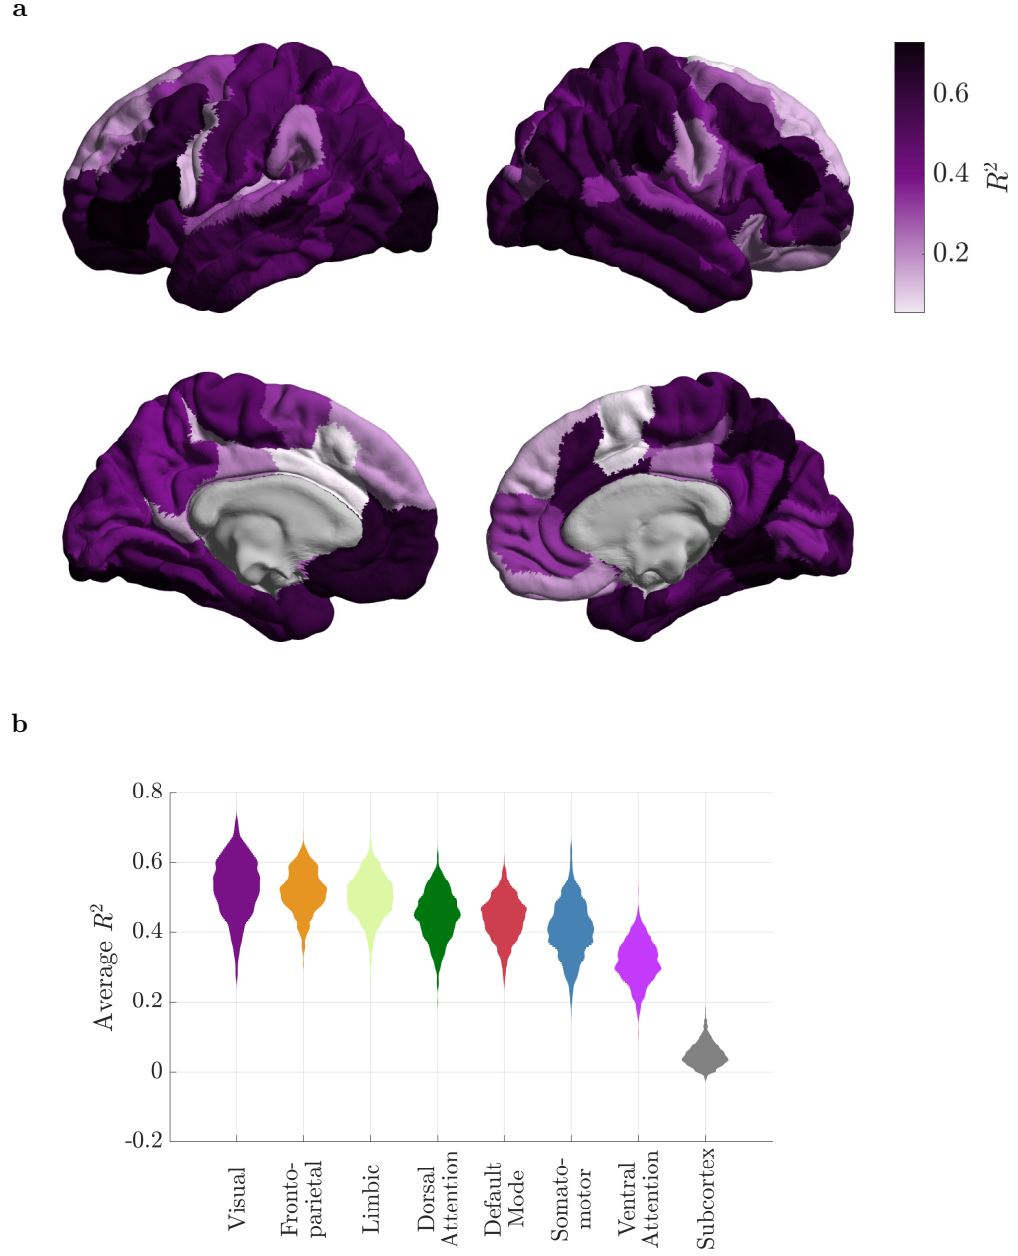

**Supplementary Figure 5: The spatial distribution of predictability.** (a) The cortical distribution of the  $R^2$  of our best model (‘VAR-3 (sparse)’), averaged over the 700 subjects. (b) Violin plots of the distribution of  $R^2$ , averaged over all the regions of each resting state network, for all subjects. Note that each distribution in panel (b) is thus composed of 700 samples. All pairs of distributions have significantly different medians in the order plotted (one-sided Mann-Whitney  $U$ -test at  $\alpha = 0.05$  with BH-FDR correction for multiple comparisons). The most striking difference is between the cortical and subcortical regions, where the dynamics of the latter are remarkably less predictable than the former. This lower predictability can be viewed as having “more noisy” dynamics or, more precisely, less spatially and temporally correlated (i.e., more white) fMRI time series in these regions.

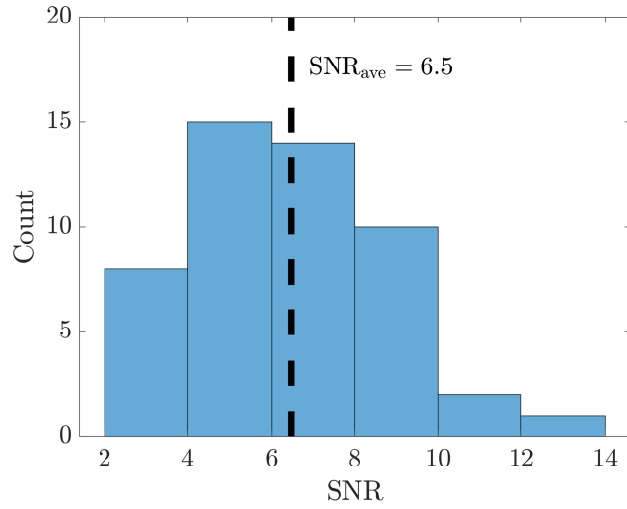

**Supplementary Figure 6: Histogram of scanner SNR estimates for rsfMRI data.** Scanner SNR was estimated for 50 randomly selected rest scans by comparing the average signal powers inside the respective subject's gray matter and outside of their head (see Methods). Due to the conservatism of this method, the resulting SNR estimates are expectedly over-estimated, but yet are not far from the  $\text{SNR} = 1$  level that is enough to completely mask nonlinear interactions on its own (Figure 4g-h).
